# Supplementary material for: Universal temperature-dependent power law excitation gaps in frustrated quantum spin systems harboring order-by-disorder
Source: arXiv:2505.18253 source file (2025-05-23)
Supplement: Supplementary file 1 [file supp_mat.pdf]

# Supplemental Material for "Universal temperature-dependent power law excitation gaps in frustrated quantum spin systems harboring order-by-disorder"

Alexander Hickey,[1] Jeffrey G. Rau,[2] Subhankar Khatua,[1,2,3] and Michel J. P. Gingras[1]

[1]*Department of Physics and Astronomy, University of Waterloo, Waterloo, Ontario, N2L 3G1, Canada*

[2]*Department of Physics, University of Windsor, 401 Sunset Avenue, Windsor, Ontario, N9B 3P4, Canada*

[3]*Institute for Theoretical Solid State Physics, IFW Dresden and Würzburg-Dresden Cluster of Excellence ct.qmat, Helmholtzstr. 20, 01069 Dresden, Germany*

(Dated: Friday 23rd May, 2025)

# I. DETAILS OF SPIN WAVE THEORY

## A. Holstein-Primakoff expansion

We consider a general bilinear spin model

$$H = \frac{1}{2}\sum_{\boldsymbol{r}\boldsymbol{r}'}\sum_{\alpha\alpha'} \boldsymbol{S}^{\intercal}_{\boldsymbol{r},\alpha}\ \boldsymbol{J}_{\boldsymbol{r}-\boldsymbol{r}',\alpha\alpha'}\boldsymbol{S}_{\boldsymbol{r}',\alpha'}, \tag{S1}$$

where $r$ represents the position of a unit cell and $\alpha$ is a sublattice index. The associated spin wave theory can be obtained by expressing the spin-operators as Holstein-Primakoff bosons,

$$\boldsymbol{S}_{\boldsymbol{r},\alpha} = \left(S - n_{\boldsymbol{r},\alpha}\right)\hat{\boldsymbol{e}}_{\alpha,0} + \sqrt{S}\left[\left(1-\frac{n_{\boldsymbol{r},\alpha}}{2S}\right)^{1/2} a_{\boldsymbol{r},\alpha}\hat{\boldsymbol{e}}_{\alpha,-} + a^{\dagger}_{\boldsymbol{r}\alpha}\left(1-\frac{n_{\boldsymbol{r},\alpha}}{2S}\right)^{1/2}\hat{\boldsymbol{e}}_{\alpha,+}\right], \tag{S2}$$

where $n_{\boldsymbol{r},\alpha} = a^{\dagger}_{\boldsymbol{r},\alpha}a_{\boldsymbol{r},\alpha}$ and the vectors $\hat{\boldsymbol{e}}_{\alpha,\pm} \equiv (\hat{\boldsymbol{e}}_{\alpha,x} \pm i\hat{\boldsymbol{e}}_{\alpha,y})/\sqrt{2}$, $\hat{\boldsymbol{e}}_{\alpha,0}$ define a local reference frame with respect to the classical ordering direction $\hat{\boldsymbol{e}}_{\alpha,0}$ (i.e. $\hat{\boldsymbol{e}}_{\alpha,x}\times\hat{\boldsymbol{e}}_{\alpha,y} = \hat{\boldsymbol{e}}_{\alpha,0}$). We define the (Fourier transform of the) exchange interactions in this local frame as

$$\mathcal{J}^{\mu\nu}_{\boldsymbol{k},\alpha\beta} \equiv \sum_{\boldsymbol{\delta}} e^{i\boldsymbol{k}\cdot\boldsymbol{\delta}}\hat{\boldsymbol{e}}^{\intercal}_{\alpha,\mu}\boldsymbol{J}_{\boldsymbol{\delta},\alpha\beta}\hat{\boldsymbol{e}}_{\beta,\nu}, \tag{S3}$$

where the sum is taken over all bonds $\boldsymbol{\delta}$ between a site on sublattice $\alpha$ to a site on sublattice $\beta$. Expanding Eq. (S2) in powers of $1/S$ about an ordered state (typically a classical ground state), leads to the series representation $H = S^2\sum_{n=0}^{\infty} S^{-n/2}H_n$. The magnon interactions to $O(S^0)$ are given by

$$H_0 = N\left(1+\frac{1}{S}\right)\epsilon_{\mathrm{cl}}, \tag{S4}$$

$$H_1 = \sqrt{N_c}\sum_{\alpha}\left[L^{\alpha}a^{\dagger}_{\boldsymbol{0},\alpha} + \overline{L}^{\alpha}a_{\boldsymbol{0},\alpha}\right], \tag{S5}$$

$$H_2 = \frac{1}{2}\sum_{\boldsymbol{k}}\sum_{\alpha\beta}\left[A^{\alpha\beta}_{\boldsymbol{k}}a^{\dagger}_{\boldsymbol{k},\alpha}a_{\boldsymbol{k},\beta} + A^{\beta\alpha}_{-\boldsymbol{k}}a_{-\boldsymbol{k},\alpha}a^{\dagger}_{-\boldsymbol{k},\beta} + B^{\alpha\beta}_{\boldsymbol{k}}a^{\dagger}_{\boldsymbol{k},\alpha}a^{\dagger}_{-\boldsymbol{k},\beta} + \overline{B}^{\alpha\beta}_{\boldsymbol{k}}a_{-\boldsymbol{k},\beta}a_{\boldsymbol{k},\alpha}\right], \tag{S6}$$

$$H_3 = \frac{1}{2!\sqrt{N_c}}\sum_{\boldsymbol{k}\boldsymbol{q}}\sum_{\alpha\beta\mu}\left[T^{\alpha\beta\mu}_{\boldsymbol{k},\boldsymbol{q}}a^{\dagger}_{\boldsymbol{k},\alpha}a^{\dagger}_{\boldsymbol{q},\beta}a_{\boldsymbol{k}+\boldsymbol{q},\mu} + \overline{T}^{\alpha\beta\mu}_{\boldsymbol{k},\boldsymbol{q}}a^{\dagger}_{\boldsymbol{k}+\boldsymbol{q},\mu}a_{\boldsymbol{q},\beta}a_{\boldsymbol{k},\alpha}\right], \tag{S7}$$

$$H_4 = \frac{1}{N_c}\sum_{\boldsymbol{k}\boldsymbol{q}\boldsymbol{Q}}\sum_{\alpha\beta\mu\nu}\left[\frac{1}{(2!)^2}V^{\alpha\beta\mu\nu}_{\boldsymbol{k},\boldsymbol{q},\boldsymbol{Q}}a^{\dagger}_{\boldsymbol{k}+\boldsymbol{Q},\alpha}a^{\dagger}_{\boldsymbol{q}-\boldsymbol{Q},\beta}a_{\boldsymbol{q},\mu}a_{\boldsymbol{k},\nu} + \frac{1}{3!}\left(D^{\alpha\beta\mu\nu}_{\boldsymbol{k},\boldsymbol{q},\boldsymbol{Q}}a^{\dagger}_{\boldsymbol{k},\alpha}a^{\dagger}_{\boldsymbol{q},\beta}a^{\dagger}_{\boldsymbol{Q},\mu}a_{\boldsymbol{k}+\boldsymbol{q}+\boldsymbol{Q},\nu} + \mathrm{H.c.}\right)\right], \tag{S8}$$

where $N = N_c N_s$ is the number of spins in a system with $N_c$ primitive unit cells, $NS^2\epsilon_{\rm cl}$ is the energy of the classical configuration, and the symmetrized interaction vertices are

$$\epsilon_{\rm cl} = \frac{1}{2N_s}\sum_{\alpha\beta}\mathcal{J}^{00}_{\mathbf{0},\alpha\beta}, \tag{S9}$$

$$L^{\alpha} = \sum_{\beta}\mathcal{J}^{+0}_{\mathbf{0},\alpha\beta}, \tag{S10}$$

$$A^{\alpha\beta}_{\boldsymbol{k}} = \mathcal{J}^{+-}_{\boldsymbol{k},\alpha\beta} - \delta_{\alpha\beta}\sum_{\mu}\mathcal{J}^{00}_{\mathbf{0},\alpha\mu}, \tag{S11}$$

$$B^{\alpha\beta}_{\boldsymbol{k}} = \mathcal{J}^{++}_{\boldsymbol{k},\alpha\beta}, \tag{S12}$$

$$T^{\alpha\beta\mu}_{\boldsymbol{k}\boldsymbol{q}} = -\delta_{\beta\mu}\mathcal{J}^{+0}_{\boldsymbol{k},\alpha\beta} - \delta_{\alpha\mu}\mathcal{J}^{+0}_{\boldsymbol{q},\beta\alpha}, \tag{S13}$$

$$\begin{aligned} V^{\alpha\beta\mu\nu}_{\boldsymbol{k},\boldsymbol{q},\boldsymbol{Q}} = &\frac{1}{2}\delta_{\alpha\mu}\delta_{\beta\nu}\left(\mathcal{J}^{00}_{\boldsymbol{k}-\boldsymbol{q}+\boldsymbol{Q},\alpha\beta} + \mathcal{J}^{00}_{-\boldsymbol{k}+\boldsymbol{q}-\boldsymbol{Q},\beta\alpha}\right) + \frac{1}{2}\delta_{\alpha\nu}\delta_{\beta\mu}\left(+\mathcal{J}^{00}_{\boldsymbol{Q},\alpha\beta} + \mathcal{J}^{00}_{-\boldsymbol{Q},\beta\alpha}\right) \\ &- \frac{1}{2}\left(\delta_{\beta\mu}\delta_{\beta\nu}\mathcal{J}^{+-}_{\boldsymbol{k}+\boldsymbol{Q},\alpha\beta} + \delta_{\alpha\mu}\delta_{\alpha\nu}\mathcal{J}^{+-}_{\boldsymbol{q}-\boldsymbol{Q},\beta\alpha} + \delta_{\alpha\beta}\delta_{\alpha\nu}\mathcal{J}^{+-}_{\boldsymbol{q},\alpha\mu} + \delta_{\alpha\beta}\delta_{\alpha\mu}\mathcal{J}^{+-}_{\boldsymbol{k},\alpha\nu}\right), \end{aligned} \tag{S14}$$

$$D^{\alpha\beta\mu\nu}_{\boldsymbol{k},\boldsymbol{q},\boldsymbol{Q}} = -\frac{1}{2}\left(\delta_{\mu\beta}\delta_{\nu\beta}\mathcal{J}^{++}_{\boldsymbol{k},\alpha\beta} + \delta_{\alpha\mu}\delta_{\alpha\nu}\mathcal{J}^{++}_{\boldsymbol{q},\beta\alpha} + \delta_{\alpha\beta}\delta_{\alpha\nu}\mathcal{J}^{++}_{\boldsymbol{Q},\mu\alpha}\right). \tag{S15}$$

The one-magnon vertex $L^{\alpha}$ vanishes so long as the classical configuration energy is at a local minimum.

### B. Linear spin wave theory

The linear spin wave Hamiltonian results from truncating the Holstein-Primakoff expansion at $O(S)$ about a configuration corresponding to a classical ground state

$$H = NS(S+1)\epsilon_{\rm cl} + S\sum_{\boldsymbol{k}}\sum_{\alpha\alpha'}\left[A^{\alpha\alpha'}_{\boldsymbol{k}}a^{\dagger}_{\boldsymbol{k},\alpha}a_{\boldsymbol{k},\alpha'} + \frac{1}{2}\left(B^{\alpha\alpha'}_{\boldsymbol{k}}a^{\dagger}_{\boldsymbol{k},\alpha}a^{\dagger}_{-\boldsymbol{k},\alpha'} + \text{H.c.}\right)\right] + O(S^{1/2}). \tag{S16}$$

The linear spin wave energies and corresponding wavefunctions are determined by diagonalizing the $2N_s \times 2N_s$ boson Bogoliubov-de Gennes matrix [1]

$$\boldsymbol{\sigma}_3\boldsymbol{M}_{\boldsymbol{k}} \equiv \begin{pmatrix} \boldsymbol{A}_{\boldsymbol{k}} & \boldsymbol{B}_{\boldsymbol{k}} \\ -\boldsymbol{B}^{\dagger}_{\boldsymbol{k}} & -\boldsymbol{A}^{\intercal}_{-\boldsymbol{k}} \end{pmatrix}, \tag{S17}$$

where $\boldsymbol{\sigma}_3 = \text{diag}(\mathbb{I}, -\mathbb{I})$ is a block Pauli matrix. We may diagonalize Eq. (S17) by defining a new set of bosons $b_{\boldsymbol{k},\alpha}$, such that

$$\begin{pmatrix} \boldsymbol{a}_{\boldsymbol{k}} \\ \boldsymbol{a}^{\dagger}_{-\boldsymbol{k}} \end{pmatrix} = \mathcal{T}_{\boldsymbol{k}}\begin{pmatrix} \boldsymbol{b}_{\boldsymbol{k}} \\ \boldsymbol{b}^{\dagger}_{-\boldsymbol{k}} \end{pmatrix}. \tag{S18}$$

By requiring $\left[b_{\boldsymbol{k},\alpha}, b_{\boldsymbol{k},\beta}\right] = 0$ and $\left[b_{\boldsymbol{k},\alpha}, b^{\dagger}_{\boldsymbol{k},\beta}\right] = \delta_{\alpha\beta}$, we obtain the para-unitary condition [2]

$$\mathcal{T}_{\boldsymbol{k}}^{-1} = \boldsymbol{\sigma}_3 \mathcal{T}_{\boldsymbol{k}}^{\dagger} \boldsymbol{\sigma}_3. \tag{S19}$$

The eigenvectors of Eq. (S17) come in pairs $\boldsymbol{V}_{\boldsymbol{k},\alpha}$ and $\boldsymbol{W}_{\boldsymbol{k},\alpha} = \boldsymbol{\sigma}_1 \overline{\boldsymbol{V}}_{-\boldsymbol{k},\alpha}$ [3], with eigenvalues $\pm\epsilon_{\pm\boldsymbol{k},\alpha}$, and make up the columns of the transformation matrix, i.e.

$$\mathcal{T}_{\boldsymbol{k}} = \begin{pmatrix} | & & | & | & & | \\ \boldsymbol{V}_{\boldsymbol{k},1} & \cdots & \boldsymbol{V}_{\boldsymbol{k},N_c} & \boldsymbol{W}_{\boldsymbol{k},1} & \cdots & \boldsymbol{W}_{\boldsymbol{k},N_c} \\ | & & | & | & & | \end{pmatrix}. \tag{S20}$$

Using Eq. (S19), the eigenvectors can be normalized to satisfy the para-orthogonality conditions

$$\boldsymbol{V}^{\dagger}_{\boldsymbol{k},\alpha} \boldsymbol{\sigma_3} \boldsymbol{V}_{\boldsymbol{k},\beta} = +\delta_{\alpha\beta}, \tag{S21}$$

$$\boldsymbol{W}^{\dagger}_{\boldsymbol{k},\alpha} \boldsymbol{\sigma_3} \boldsymbol{W}_{\boldsymbol{k},\beta} = -\delta_{\alpha\beta}, \tag{S22}$$

$$\boldsymbol{V}^{\dagger}_{\boldsymbol{k},\alpha} \boldsymbol{\sigma_3} \boldsymbol{W}_{\boldsymbol{k},\beta} = 0. \tag{S23}$$

The linear spin wave Hamiltonian then takes the diagonal form

$$H = NS(S+1)\epsilon_{\text{cl}} + NS\epsilon_{\text{qu}} + \frac{S}{2} \sum_{\boldsymbol{k}} \sum_{\alpha} \epsilon_{\boldsymbol{k},\alpha} b^{\dagger}_{\boldsymbol{k},\alpha} b_{\boldsymbol{k},\alpha} + O(S^{1/2}), \tag{S24}$$

where the quantum zero-point energy (per spin) is

$$S\epsilon_{\text{qu}} \equiv \frac{S}{2N} \sum_{\boldsymbol{k}} \sum_{\alpha} \epsilon_{\boldsymbol{k},\alpha}. \tag{S25}$$

We may subsequently calculate the free energy (per spin) to $O(S)$ at temperature $T$ as

$$f(T) = S(S+1)\epsilon_{\text{cl}} + S\epsilon_{\text{qu}} + \frac{k_{\text{B}}T}{N} \sum_{\boldsymbol{k}} \sum_{\alpha} \ln\left(1 - e^{-S\epsilon_{\boldsymbol{k},\alpha}/k_{\text{B}}T}\right) + O(S^{1/2}). \tag{S26}$$

Next, we discuss the circumstance of interest, where the linear spin wave spectrum contains zero modes. This implies that the matrix $\boldsymbol{\sigma}_3 \boldsymbol{M}_{\boldsymbol{k}}$ is positive *semi-definite*. We assume, without loss of generality, that there is a single zero mode at the Brillouin zone center ($\boldsymbol{k} = \boldsymbol{0}$). This mode can be classified based on the spectral properties of $\boldsymbol{M}_0 \equiv \boldsymbol{M}_{\boldsymbol{0}}$. In particular, $\boldsymbol{M}_0$ has either one or two linearly independent eigenvectors corresponding to the zero mode, which we refer to as *type I* and *type II* respectively. We define $\boldsymbol{V}_0$ and $\boldsymbol{W}_0$ to be the vectors that span the zero mode subspace, while simultaneously satisfying the normalization conditions Eqs. (S21-S23). The projection of $\boldsymbol{M}_0$ into

the zero mode subspace is then given by [4]

$$\begin{pmatrix} \boldsymbol{V}_0^\dagger \boldsymbol{M_0} \boldsymbol{V}_0 & \boldsymbol{V}_0^\dagger \boldsymbol{M_0} \boldsymbol{W}_0 \\ \boldsymbol{W}_0^\dagger \boldsymbol{M_0} \boldsymbol{V}_0 & \boldsymbol{W}_0^\dagger \boldsymbol{M_0} \boldsymbol{W}_0 \end{pmatrix} = \begin{cases} \boldsymbol{V}_0^\dagger \boldsymbol{M_0} \boldsymbol{V}_0 \begin{pmatrix} 1 & 1 \\ 1 & 1 \end{pmatrix} & \text{(type I)} \\ \begin{pmatrix} 0 & 0 \\ 0 & 0 \end{pmatrix} & \text{(type II)} \end{cases} . \tag{S27}$$

A more detailed treatment of non-interacting bosons with zero modes can be found in Refs. [1, 4].

### C. Non-linear spin wave theory at finite temperature

To incorporate effects of spin wave interactions at leading order in $1/S$ and at finite temperature, we use the imaginary time formalism. To this effect, we assume the $O(S)$ Hamiltonian in Eq. (S16) is solvable, and treat the three- and four-body interactions perturbatively to $O(S^0)$ [5]. We are interested in the single-magnon spectrum, encoded in the thermal Green's functions

$$\mathcal{G}^{-+}_{\alpha\beta}(\boldsymbol{k}, i\omega_n) = \int_0^{(k_\mathrm{B}T)^{-1}} \mathrm{d}\tau\, e^{i\omega_n \tau} \left\langle \mathbb{T} a_{\boldsymbol{k},\alpha}(\tau) a^\dagger_{\boldsymbol{k},\beta}(0) \right\rangle, \tag{S28}$$

$$\mathcal{G}^{+-}_{\alpha\beta}(\boldsymbol{k}, i\omega_n) = \int_0^{(k_\mathrm{B}T)^{-1}} \mathrm{d}\tau\, e^{i\omega_n \tau} \left\langle \mathbb{T} a^\dagger_{-\boldsymbol{k},\alpha}(\tau) a_{-\boldsymbol{k},\beta}(0) \right\rangle, \tag{S29}$$

$$\mathcal{G}^{++}_{\alpha\beta}(\boldsymbol{k}, i\omega_n) = \int_0^{(k_\mathrm{B}T)^{-1}} \mathrm{d}\tau\, e^{i\omega_n \tau} \left\langle \mathbb{T} a^\dagger_{-\boldsymbol{k},\alpha}(\tau) a^\dagger_{\boldsymbol{k},\beta}(0) \right\rangle, \tag{S30}$$

$$\mathcal{G}^{--}_{\alpha\beta}(\boldsymbol{k}, i\omega_n) = \int_0^{(k_\mathrm{B}T)^{-1}} \mathrm{d}\tau\, e^{i\omega_n \tau} \left\langle \mathbb{T} a_{\boldsymbol{k},\alpha}(\tau) a_{-\boldsymbol{k},\beta}(0) \right\rangle, \tag{S31}$$

where $\alpha, \beta$ label the sublattice structure, $\omega_n = \frac{2\pi n}{k_\mathrm{B}T}$ is a bosonic Matsubara frequency, $\mathbb{T}$ is the (imaginary) time-ordering operator [6], $\langle \cdots \rangle$ denotes the thermal average with respect to the equilibrium density matrix $\rho = Z^{-1} e^{-H/k_\mathrm{B}T}$ [7]. This can be organized more compactly into a Bogoliubov-de Gennes block matrix, analogous to Eq. (S17)

$$\boldsymbol{\mathcal{G}}(\boldsymbol{k}, i\omega_n) \equiv \begin{pmatrix} \mathcal{G}^{-+}(\boldsymbol{k}, i\omega_n) & \mathcal{G}^{--}(\boldsymbol{k}, i\omega_n) \\ \mathcal{G}^{++}(\boldsymbol{k}, i\omega_n) & \mathcal{G}^{+-}(\boldsymbol{k}, i\omega_n) \end{pmatrix} = \Big[ -i\omega_n + \boldsymbol{\sigma}_3 \left( S\boldsymbol{M}_{\boldsymbol{k}} + \boldsymbol{\Sigma}(\boldsymbol{k}, i\omega_n) \right) \Big]^{-1} \boldsymbol{\sigma}_3, \tag{S32}$$

where $\boldsymbol{\Sigma}(\boldsymbol{k}, i\omega_n)$ is the imaginary time self-energy that encodes interactions. The single-magnon dispersion then corresponds to poles of the (real time) retarded Green's function, related to the thermal Green's function via analytic continuation

$$\boldsymbol{G}^\mathrm{R}(\boldsymbol{k}, \omega) = -\boldsymbol{\mathcal{G}}(\boldsymbol{k}, i\omega_n \to \omega + i0^+) = \Big[ \omega + i0^+ - \boldsymbol{\sigma}_3 \left( S\boldsymbol{M}_{\boldsymbol{k}} + \boldsymbol{\Sigma}^\mathrm{R}(\boldsymbol{k}, \omega) \right) \Big]^{-1} \boldsymbol{\sigma}_3, \tag{S33}$$

with the retarded self-energy defined similarly as $\boldsymbol{\Sigma}^{\mathrm{R}}(\boldsymbol{k},\omega) = \boldsymbol{\Sigma}(\boldsymbol{k}, i\omega_n \to \omega + i0^+)$. We note that the temperature dependence of Eq. (S33) enters implicitly in the self-energy.

### D. Calculation of the pseudo-Goldstone gap

For the remainder of Sec. I, the calculation of the pseudo-Goldstone (PG) gap proceeds similarly to Ref. [4], but now with the retarded self-energy $\boldsymbol{\Sigma}^{\mathrm{R}}(\boldsymbol{k},\omega)$ evaluated at finite temperature $T$. Since the PG mode appears at zero energy in linear spin-wave theory, we may expand the self energy to leading order

$$\boldsymbol{\Sigma}^{\mathrm{R}}(\mathbf{0},\omega) = \boldsymbol{\Sigma}^{\mathrm{R}}(\mathbf{0},0) + O(S^{-1}), \tag{S34}$$

which is exact to $O(S^0)$. The subspace associated with the PG mode is two-dimensional, therefore we must calculate the poles of Eq. (S33) in the context of degenerate perturbation theory. At $O(S^0)$, this comes down to diagonalizing the effective Hamiltonian [4]

$$H_{\mathrm{eff}} \equiv \boldsymbol{\sigma}_3 \begin{pmatrix} \boldsymbol{V}_0^\dagger \left[ S\boldsymbol{M}_\mathbf{0} + \boldsymbol{\Sigma}_0^{\mathrm{R}}(T) \right] \boldsymbol{V}_0 & \boldsymbol{V}_0^\dagger \left[ S\boldsymbol{M}_\mathbf{0} + \boldsymbol{\Sigma}_0^{\mathrm{R}}(T) \right] \boldsymbol{W}_0 \\ \boldsymbol{W}_0^\dagger \left[ S\boldsymbol{M}_\mathbf{0} + \boldsymbol{\Sigma}_0^{\mathrm{R}}(T) \right] \boldsymbol{V}_0 & \boldsymbol{W}_0^\dagger \left[ S\boldsymbol{M}_\mathbf{0} + \boldsymbol{\Sigma}_0^{\mathrm{R}}(T) \right] \boldsymbol{W}_0 \end{pmatrix} \tag{S35}$$

projected into the zero mode subspace, where we have defined $\boldsymbol{\Sigma}_0^{\mathrm{R}}(T) \equiv \boldsymbol{\Sigma}^{\mathrm{R}}(\mathbf{0},0)$ to make the temperature dependence explicit. In the case of a type I mode, we may use Eq. (S27) to compute the effective Hamiltonian

$$H_{\mathrm{eff}} = \begin{pmatrix} S\boldsymbol{V}_0^\dagger \boldsymbol{M}_\mathbf{0} \boldsymbol{V}_0 + \boldsymbol{V}_0^\dagger \boldsymbol{\Sigma}_0^{\mathrm{R}}(T) \boldsymbol{V}_0 & S\boldsymbol{V}_0^\dagger \boldsymbol{M}_\mathbf{0} \boldsymbol{V}_0 + \boldsymbol{V}_0^\dagger \boldsymbol{\Sigma}_0^{\mathrm{R}}(T) \boldsymbol{W}_0 \\ -S\boldsymbol{V}_0^\dagger \boldsymbol{M}_\mathbf{0} \boldsymbol{V}_0 - \boldsymbol{W}_0^\dagger \boldsymbol{\Sigma}_0^{\mathrm{R}}(T) \boldsymbol{V}_0 & -S\boldsymbol{V}_0^\dagger \boldsymbol{M}_\mathbf{0} \boldsymbol{V}_0 - \boldsymbol{V}_0^\dagger \boldsymbol{\Sigma}_0^{\mathrm{R}}(T) \boldsymbol{V}_0 \end{pmatrix}. \tag{S36}$$

Computing the eigenvalues of $H_{\mathrm{eff}}$, we obtain a PG gap of $O(S^{1/2})$,

$$\Delta(T) = S^{1/2} \sqrt{\boldsymbol{V}_0^\dagger \left[ \boldsymbol{\Sigma}_0^{\mathrm{R}}(T) \boldsymbol{\sigma}_3 \boldsymbol{M}_\mathbf{0} + \boldsymbol{M}_\mathbf{0} \boldsymbol{\sigma}_3 \boldsymbol{\Sigma}_0^{\mathrm{R}}(T) \right] \boldsymbol{V}_0}. \tag{S37}$$

Similarly, for a type II mode, we use Eq. (S27) to obtain

$$H_{\mathrm{eff}} = \begin{pmatrix} \boldsymbol{V}_0^\dagger \boldsymbol{\Sigma}_0^{\mathrm{R}}(T) \boldsymbol{V}_0 & \boldsymbol{V}_0^\dagger \boldsymbol{\Sigma}_0^{\mathrm{R}}(T) \boldsymbol{W}_0 \\ -\boldsymbol{W}_0^\dagger \boldsymbol{\Sigma}_0^{\mathrm{R}}(T) \boldsymbol{V}_0 & -\boldsymbol{W}_0^\dagger \boldsymbol{\Sigma}_0^{\mathrm{R}}(T) \boldsymbol{W}_0 \end{pmatrix}. \tag{S38}$$

In this case, the PG gap appears at $O(S^0)$ as

$$\Delta(T) = S^0 \sqrt{\left( \boldsymbol{V}_0^\dagger \boldsymbol{\Sigma}_0^{\mathrm{R}}(T) \boldsymbol{V}_0 \right)^2 - \left| \boldsymbol{V}_0^\dagger \boldsymbol{\Sigma}_0^{\mathrm{R}}(T) \boldsymbol{W}_0 \right|^2}. \tag{S39}$$

## II. CURVATURE FORMULA

Next, we show how the PG gap computed to $O(S^0)$, at finite temperature, can be related to the curvatures of the linear spin-wave dispersion. This is in essence a nonzero temperature generalization of the curvature formula derived in Ref. [4], where it was shown that the relationship between these two quantities can be established through the first moment of the magnon spectral function, projected into the zero-mode subspace. We consider the Holstein-Primakoff expansion about a configuration that is related to the classical ground state by small rotations about the local $\hat{\boldsymbol{e}}_{\alpha,x}$ and $\hat{\boldsymbol{e}}_{\alpha,y}$ axes, labeled by the angles $\theta$ and $\phi$ respectively. Relative to the classical ground state, this transforms the local frame as

$$\hat{\boldsymbol{e}}_{\alpha,0}(\zeta) = \left(1 - |\zeta|^2\right)\hat{\boldsymbol{e}}_{\alpha,0} + \bar{\zeta}\hat{\boldsymbol{e}}_{\alpha,+} + \zeta\hat{\boldsymbol{e}}_{\alpha,-} + O(\zeta^3), \tag{S40}$$

$$\hat{\boldsymbol{e}}_{\alpha,+}(\zeta) = \left(1 - \frac{1}{2}|\zeta|^2 + \frac{1}{4}\bar{\zeta}^2 - \frac{1}{4}\zeta^2\right)\hat{\boldsymbol{e}}_{\alpha,+} - \zeta\hat{\boldsymbol{e}}_{\alpha,0} - \frac{1}{4}\zeta^2\hat{\boldsymbol{e}}_{\alpha,-} + O(\zeta^3), \tag{S41}$$

$$\hat{\boldsymbol{e}}_{\alpha,-}(\zeta) = \left(1 - \frac{1}{2}|\zeta|^2 + \frac{1}{4}\zeta^2 - \frac{1}{4}\bar{\zeta}^2\right)\hat{\boldsymbol{e}}_{\alpha,-} - \bar{\zeta}\hat{\boldsymbol{e}}_{\alpha,0} - \frac{1}{4}\bar{\zeta}^2\hat{\boldsymbol{e}}_{\alpha,+} + O(\zeta^3), \tag{S42}$$

where $\zeta \equiv (\phi + i\theta)/\sqrt{2}$. One can subsequently calculate the appropriate spin-wave theory using Eqs. (S4-S8). Alternatively, these small rotations can be related to the magnon zero-modes

$$b_0 \equiv \boldsymbol{V}_0^\dagger\boldsymbol{\sigma}_3\begin{pmatrix}\boldsymbol{a_0}\\ \boldsymbol{a_0}^\dagger\end{pmatrix}, \qquad b_0^\dagger \equiv -\boldsymbol{W}_0^\dagger\boldsymbol{\sigma}_3\begin{pmatrix}\boldsymbol{a_0}\\ \boldsymbol{a_0}^\dagger\end{pmatrix}, \tag{S43}$$

using the Hermitian operators

$$\Phi \equiv \sqrt{\frac{SN}{2}}\left[b_0^\dagger + b_0\right] + O(S^{-1/2}) \tag{S44}$$

$$\Theta \equiv i\sqrt{\frac{SN}{2}}\left[b_0^\dagger - b_0\right] + O(S^{-1/2}). \tag{S45}$$

These operators generate rotations about the soft directions [4], given by the unitary operator

$$U(\phi,\theta) \equiv e^{-i\phi\Phi}e^{-i\theta\Theta}. \tag{S46}$$

This can be used to define a transformed Hamiltonian that encodes these rotations $\mathcal{H}(\phi,\theta) \equiv U(\phi,\theta)^\dagger H U(\phi,\theta)$. Expanding to second order in $\phi$ and $\theta$ using the Baker–Campbell–Hausdorff formula, we obtain

$$\mathcal{H}(\phi,\theta) = H + i\theta[\Theta,H] + i\phi[\Phi,H] - \frac{1}{2}\theta^2[\Theta,[\Theta,H]] - \frac{1}{2}\phi^2[\Phi,[\Phi,H]] - \phi\theta[\Phi,[\Theta,H]] + O(\zeta^3). \tag{S47}$$

Proceeding to compute the curvatures of $\mathcal{H}(\phi,\theta)$, we find they are related to the nested commutators

$$\left(\frac{\partial^2\mathcal{H}}{\partial\phi^2}\right)_0 = -[\Phi,[\Phi,H]], \qquad \left(\frac{\partial^2\mathcal{H}}{\partial\theta^2}\right)_0 = -[\Theta,[\Theta,H]], \qquad \left(\frac{\partial^2\mathcal{H}}{\partial\phi\partial\theta}\right)_0 = \left(\frac{\partial^2\mathcal{H}}{\partial\theta\partial\phi}\right)_0 = -[\Phi,[\Theta,H]], \tag{S48}$$

where $(\cdots)_0$ is used as a shorthand for the evaluation at $\phi=\theta=0$.

### A. First moment of the spectral function

To relate the curvatures in Eqs. (S48) to the PG gap, we first establish a sum rule for the first moment of the magnon spectral function. More generally, the real-time retarded and advanced Green's function for a pair of operators $X$ and $Y$ are respectively [6]

$$G^{\mathrm{R}}_{XY}(t) \equiv -i\theta(t)\left\langle [X(t),Y(0)]\right\rangle, \tag{S49}$$

$$G^{\mathrm{A}}_{XY}(t) \equiv i\theta(-t)\left\langle [X(t),Y(0)]\right\rangle, \tag{S50}$$

with $\theta(t)$ the Heaviside step function and the time evolution is assumed to be in the Heisenberg picture, i.e. $\frac{\mathrm{d}X}{\mathrm{d}t} = i[H,X]$. The corresponding spectral function is defined as

$$\mathcal{A}_{XY}(\omega) \equiv \frac{1}{2i}\int_{-\infty}^{\infty}\mathrm{d}t\, e^{i\omega t}\left[G^{\mathrm{R}}_{XY}(t) - G^{\mathrm{A}}_{XY}(t)\right]. \tag{S51}$$

The first moment of this spectral function is then

$$\int_{-\infty}^{\infty}\mathrm{d}\omega\,\omega\mathcal{A}_{XY}(\omega) = \frac{1}{2}\int_{-\infty}^{\infty}\mathrm{d}\omega\int_{-\infty}^{\infty}\mathrm{d}t\, e^{i\omega t}\frac{\mathrm{d}}{\mathrm{d}t}\left[G^{\mathrm{R}}_{XY}(t) - G^{\mathrm{A}}_{XY}(t)\right] = -\left\langle [Y,[X,H]]\right\rangle \tag{S52}$$

The following sum rules then directly follow from Eqs. (S48)

$$\int_{-\infty}^{\infty}\mathrm{d}\omega\,\omega\mathcal{A}_{\Phi\Phi}(\omega) = \left\langle\left(\frac{\partial^2\mathcal{H}}{\partial\phi^2}\right)_0\right\rangle, \qquad \int_{-\infty}^{\infty}\mathrm{d}\omega\,\omega\mathcal{A}_{\Theta\Theta}(\omega) = \left\langle\left(\frac{\partial^2\mathcal{H}}{\partial\theta^2}\right)_0\right\rangle, \tag{S53}$$

$$\int_{-\infty}^{\infty}\mathrm{d}\omega\,\omega\mathcal{A}_{\Phi\Theta}(\omega) = \left\langle\left(\frac{\partial^2\mathcal{H}}{\partial\phi\partial\theta}\right)_0\right\rangle, \qquad \int_{-\infty}^{\infty}\mathrm{d}\omega\,\omega\mathcal{A}_{\Theta\Phi}(\omega) = \left\langle\left(\frac{\partial^2\mathcal{H}}{\partial\theta\partial\phi}\right)_0\right\rangle. \tag{S54}$$

Next, we relate these spectral functions to the single magnon spectral function, defined using Eq. (S33) as

$$\boldsymbol{\mathcal{A}}(\boldsymbol{k},\omega) = \frac{1}{2i}\left[\boldsymbol{G}^{\mathrm{R}}(\boldsymbol{k},\omega) - \boldsymbol{G}^{\mathrm{R}}(\boldsymbol{k},\omega)^\dagger\right], \tag{S55}$$

Projecting into the zero mode subspace, using Eq. S43, we find

$$\boldsymbol{\mathcal{A}}_0(\omega) \equiv \begin{pmatrix} \mathcal{A}_{b_0 b_0^\dagger}(\omega) & \mathcal{A}_{b_0 b_0}(\omega) \\ \mathcal{A}_{b_0^\dagger b_0^\dagger}(\omega) & \mathcal{A}_{b_0^\dagger b_0}(\omega) \end{pmatrix} = \begin{pmatrix} \boldsymbol{V}_0^\dagger\boldsymbol{\sigma}_3\boldsymbol{\mathcal{A}}(\boldsymbol{0},\omega)\boldsymbol{\sigma}_3\boldsymbol{V}_0 & -\boldsymbol{V}_0^\dagger\boldsymbol{\sigma}_3\boldsymbol{\mathcal{A}}(\boldsymbol{0},\omega)\boldsymbol{\sigma}_3\boldsymbol{W}_0 \\ -\boldsymbol{W}_0^\dagger\boldsymbol{\sigma}_3\boldsymbol{\mathcal{A}}(\boldsymbol{0},\omega)\boldsymbol{\sigma}_3\boldsymbol{V}_0 & \boldsymbol{W}_0^\dagger\boldsymbol{\sigma}_3\boldsymbol{\mathcal{A}}(\boldsymbol{0},\omega)\boldsymbol{\sigma}_3\boldsymbol{W}_0 \end{pmatrix}. \tag{S56}$$

We can make use of Eqs. (S44-S45) and the rotated vectors

$$\boldsymbol{U}_\phi \equiv \frac{i}{\sqrt{2}}\left(\boldsymbol{W}_0 - \boldsymbol{V}_0\right), \qquad \boldsymbol{U}_\theta \equiv \frac{1}{\sqrt{2}}\left(\boldsymbol{W}_0 + \boldsymbol{V}_0\right), \tag{S57}$$

to write the spectral functions of $\Phi$ and $\Theta$ as

$$\mathcal{A}_{\mu\nu}(\omega) = NS\boldsymbol{U}_\mu^\dagger \boldsymbol{\sigma}_3 \boldsymbol{\mathcal{A}}(\boldsymbol{0},\omega)\boldsymbol{\sigma}_3 \boldsymbol{U}_\nu, \tag{S58}$$

where $\mu,\nu = \Phi,\Theta$. The first moment of the magnon spectral functions may then be written in the compact form

$$\frac{1}{SN}\left\langle\left(\frac{\partial^2\mathcal{H}}{\partial\lambda_\mu\partial\lambda_\nu}\right)_0\right\rangle = \boldsymbol{U}_\mu^\dagger\boldsymbol{\sigma}_3\left[\int_{-\infty}^{\infty} \mathrm{d}\omega\, \omega\, \boldsymbol{\mathcal{A}}(\boldsymbol{0},\omega)\right]\boldsymbol{\sigma}_3\boldsymbol{U}_\nu, \tag{S59}$$

where $\lambda_\Phi \equiv \phi$ and $\lambda_\Theta \equiv \theta$. This is equivalent to the result derived in [4], with the expectation value now performed at nonzero temperature $T$. It is also useful to express the Eq. (S59) in terms of the zero mode magnons explicitly. It follows from Eqs. (S44-S45) that

$$\boldsymbol{\mathcal{A}}_0(\omega) = \frac{1}{2SN}\Big[(1+\boldsymbol{\sigma}_1)\mathcal{A}_{\Phi\Phi}(\omega) + (1-\boldsymbol{\sigma}_1)\mathcal{A}_{\Theta\Theta}(\omega) - (\boldsymbol{\sigma}_2 + i\boldsymbol{\sigma}_3)\mathcal{A}_{\Phi\Theta}(\omega) - (\boldsymbol{\sigma}_2 - i\boldsymbol{\sigma}_3)\mathcal{A}_{\Theta\Phi}(\omega)\Big]. \tag{S60}$$

This implies that the first moment can be written as

$$\int_{-\infty}^{\infty}\mathrm{d}\omega\,\omega\boldsymbol{\mathcal{A}}_0(\omega) = \frac{1}{2SN}\left[(1+\boldsymbol{\sigma}_1)\left\langle\left(\frac{\partial^2\mathcal{H}}{\partial\phi^2}\right)_0\right\rangle + (1-\boldsymbol{\sigma}_1)\left\langle\left(\frac{\partial^2\mathcal{H}}{\partial\theta^2}\right)_0\right\rangle - 2\boldsymbol{\sigma}_2\left\langle\left(\frac{\partial^2\mathcal{H}}{\partial\phi\partial\theta}\right)_0\right\rangle\right]. \tag{S61}$$

This sum rule will enable us to demonstrate the equivalence between the PG gap and the curvature formula in the main text.

### B. Calculation of the gap

Next, we discuss how to use the sum rule to calculate the PG gap for both type I and type II modes. Using Eqs. (S40-S42), we carry out a Holstein-Primakoff expansion about a rotated spin configuration to obtain $\mathcal{H}(\phi,\theta)$. First, we discuss the case of a type II PG mode, where both angles $\phi$ and $\theta$ correspond to soft directions. In this case, the Holstein-Primakoff expansion is

$$\mathcal{H}(\phi,\theta) = S(S+1)N\epsilon_{\mathrm{cl}} + SN\epsilon_{\mathrm{qu}}(\phi,\theta) + S\sum_{\boldsymbol{k},\alpha}\epsilon_{\boldsymbol{k},\alpha}(\phi,\theta)b^\dagger_{\boldsymbol{k},\alpha}b_{\boldsymbol{k},\alpha} + O(S^{1/2}),$$

as the classical configuration energy $\epsilon_{\mathrm{cl}}$ is independent of $\phi$ and $\theta$. The second derivative is then [4]

$$\frac{1}{SN}\left\langle\left(\frac{\partial^2\mathcal{H}}{\partial\lambda_\mu\partial\lambda_\nu}\right)_0\right\rangle = \left(\frac{\partial^2\epsilon_{\mathrm{qu}}}{\partial\lambda_\mu\partial\lambda_\nu}\right)_0 + \frac{1}{N}\sum_{\boldsymbol{k}}\sum_{\alpha}\left(\frac{\partial^2\epsilon_{\boldsymbol{k}\alpha}}{\partial\lambda_\mu\partial\lambda_\nu}\right)_0 n_{\mathrm{B}}(\epsilon_{\boldsymbol{k},\alpha}) + O(S^{-1}), \tag{S62}$$

where $n_{\mathrm{B}}(\epsilon_{\boldsymbol{k},\alpha}) \equiv \left(\exp\left(\frac{S\epsilon_{\boldsymbol{k},\alpha}}{k_{\mathrm{B}}T}\right) - 1\right)^{-1}$ is the Bose distribution function. Eq. (S62) can be written in a more tractable form involving the free energy per spin, defined as

$$f(\phi,\theta) = S(S+1)\epsilon_{\mathrm{cl}} + S\epsilon_{\mathrm{qu}}(\phi,\theta) + \frac{k_{\mathrm{B}}T}{N}\sum_{\boldsymbol{k}}\sum_{\alpha}\ln\left(1 - e^{-S\epsilon_{\boldsymbol{k},\alpha}(\phi,\theta)/k_{\mathrm{B}}T}\right). \tag{S63}$$

It follows that

$$g_{\mu\nu} \equiv \frac{1}{SN}\left\langle\left(\frac{\partial^2\mathcal{H}}{\partial\lambda_\mu\partial\lambda_\nu}\right)_0\right\rangle = \frac{1}{S}\left[\left(\frac{\partial^2 f}{\partial\lambda_\mu\partial\lambda_\nu}\right)_0 + K_{\mu\nu}\right], \tag{S64}$$

where

$$K_{\mu\nu} \equiv \frac{S^2}{4k_{\mathrm{B}}TN}\sum_{\boldsymbol{k},\alpha}\left(\frac{\partial\epsilon_{\boldsymbol{k},\alpha}}{\partial\lambda_\mu}\right)_0\left(\frac{\partial\epsilon_{\boldsymbol{k},\alpha}}{\partial\lambda_\nu}\right)_0 \operatorname{csch}^2\left(\frac{S\epsilon_{\boldsymbol{k},\alpha}}{2k_{\mathrm{B}}T}\right). \tag{S65}$$

To calculate the PG gap, we use the fact that the first moment of the spectral function is *equivalent* to the effective Hamiltonian in Eq. (S35) (see Ref. [4] for more details). In particular, we have

$$\boldsymbol{\sigma}_3\int_{-\infty}^{\infty} \mathrm{d}\omega\,\omega\mathcal{A}_0(\omega) = H_{\mathrm{eff}} = \frac{1}{2}\begin{pmatrix} g_{\Theta\Theta} + g_{\Phi\Phi} & g_{\Theta\Theta} - g_{\Phi\Phi} + 2ig_{\Phi\Theta} \\ g_{\Phi\Phi} - g_{\Theta\Theta} + 2ig_{\Phi\Theta} & -g_{\Theta\Theta} - g_{\Phi\Phi}\end{pmatrix}. \tag{S66}$$

Diagonalizing $H_{\mathrm{eff}}$, we find for the PG gap

$$\Delta(T) = S^0\sqrt{g_{\Theta\Theta}g_{\Phi\Phi} - g_{\Phi\Theta}^2} \qquad \text{(Type II)}. \tag{S67}$$

Next, we consider the case of a type I PG mode, where only one of the angles $\phi$ corresponds to a soft direction. In this case, the Holstein-Primakoff expansion is only stable when $\theta = 0$. Following the same line of reasoning as Ref. [4], we find

$$\boldsymbol{\sigma}_3\int_{-\infty}^{\infty} \mathrm{d}\omega\,\omega\mathcal{A}_0(\omega) = H_{\mathrm{eff}} = \frac{1}{2}\begin{pmatrix} S\left(\frac{\partial^2\epsilon_{\mathrm{cl}}}{\partial\theta^2}\right)_0 + g_{\Phi\Phi} & S\left(\frac{\partial^2\epsilon_{\mathrm{cl}}}{\partial\theta^2}\right)_0 - g_{\Phi\Phi} \\ g_{\Phi\Phi} - S\left(\frac{\partial^2\epsilon_{\mathrm{cl}}}{\partial\theta^2}\right)_0 & -S\left(\frac{\partial^2\epsilon_{\mathrm{cl}}}{\partial\theta^2}\right)_0 - g_{\Phi\Phi}\end{pmatrix}. \tag{S68}$$

Diagonalizing $H_{\mathrm{eff}}$, we find for the PG gap

$$\Delta(T) = S^{1/2}\sqrt{\left(\frac{\partial^2\epsilon_{\mathrm{cl}}}{\partial\theta^2}\right)_0 g_{\Phi\Phi}} \qquad \text{(Type I)}. \tag{S69}$$

### C. Evaluation of $K_{\mu\nu}$

In this subsection, we discuss the evaluation of Eq. (S65) and the circumstances when this term vanishes. One can work out an explicit form of these derivatives with respect to the spin exchange matrices in a local reference frame, avoiding the need to approximate them numerically. For this,

we make use of the Hellmann-Feynmann theorem, generalized to bosonic Bogoliubov-de Gennes systems.

To begin, suppose the spin-wave theory depends on some continuous parameter $\lambda$. The linear spin-wave energies satisfy the eigenvalue equation $\boldsymbol{\sigma}_3\boldsymbol{M}_{\boldsymbol{k}}(\lambda)\boldsymbol{V}_{\boldsymbol{k},\alpha}(\lambda) = \epsilon_{\boldsymbol{k},\alpha}(\lambda)\boldsymbol{V}_{\boldsymbol{k},\alpha}(\lambda)$. So long as the normalization conditions Eqs. (S21-S23) are satisfied, the derivatives of the spin-wave energies satisfy

$$\frac{\partial\epsilon_{\boldsymbol{k},\alpha}}{\partial\lambda} = \boldsymbol{V}^{\dagger}_{\boldsymbol{k},\alpha}\frac{\partial\boldsymbol{M}_{\boldsymbol{k}}}{\partial\lambda}\boldsymbol{V}_{\boldsymbol{k},\alpha}. \tag{S70}$$

Making use of the local rotated frame in Eqs. (S40-S42), the first derivatives are evaluated to

$$\begin{aligned}
\left(\frac{\partial\hat{\boldsymbol{e}}_{a,0}}{\partial\theta}\right)_0 &= -\frac{i}{\sqrt{2}}\left(\hat{\boldsymbol{e}}_{a,+} - \hat{\boldsymbol{e}}_{a,-}\right), & \left(\frac{\partial\hat{\boldsymbol{e}}_{a,+}}{\partial\theta}\right)_0 &= -\frac{i}{\sqrt{2}}\hat{\boldsymbol{e}}_{a,0}, & \left(\frac{\partial\hat{\boldsymbol{e}}_{a,-}}{\partial\theta}\right)_0 &= +\frac{i}{\sqrt{2}}\hat{\boldsymbol{e}}_{a,0},\\
\left(\frac{\partial\hat{\boldsymbol{e}}_{a,0}}{\partial\phi}\right)_0 &= +\frac{1}{\sqrt{2}}\left(\hat{\boldsymbol{e}}_{a,+} + \hat{\boldsymbol{e}}_{a,-}\right), & \left(\frac{\partial\hat{\boldsymbol{e}}_{a,+}}{\partial\phi}\right)_0 &= -\frac{1}{\sqrt{2}}\hat{\boldsymbol{e}}_{a,0}, & \left(\frac{\partial\hat{\boldsymbol{e}}_{a,-}}{\partial\phi}\right)_0 &= -\frac{1}{\sqrt{2}}\hat{\boldsymbol{e}}_{a,0}.
\end{aligned} \tag{S71}$$

It follows that the local exchange matrices are given by

$$\begin{aligned}
\left(\frac{\partial\mathcal{J}^{+-}_{\boldsymbol{k},\alpha\beta}}{\partial\theta}\right)_0 &= +\frac{i}{\sqrt{2}}\left(\mathcal{J}^{+0}_{\boldsymbol{k},\alpha\beta} - \bar{\mathcal{J}}^{+0}_{\boldsymbol{k},\beta\alpha}\right), & \left(\frac{\partial\mathcal{J}^{++}_{\boldsymbol{k},\alpha\beta}}{\partial\theta}\right)_0 &= -\frac{i}{\sqrt{2}}\left(\mathcal{J}^{+0}_{\boldsymbol{k},\alpha\beta} + \mathcal{J}^{+0}_{-\boldsymbol{k},\beta\alpha}\right),\\
\left(\frac{\partial\mathcal{J}^{+-}_{\boldsymbol{k},\alpha\beta}}{\partial\phi}\right)_0 &= -\frac{1}{\sqrt{2}}\left(\mathcal{J}^{+0}_{\boldsymbol{k},\alpha\beta} + \bar{\mathcal{J}}^{+0}_{\boldsymbol{k},\beta\alpha}\right), & \left(\frac{\partial\mathcal{J}^{++}_{\boldsymbol{k},\alpha\beta}}{\partial\phi}\right)_0 &= -\frac{1}{\sqrt{2}}\left(\mathcal{J}^{+0}_{\boldsymbol{k},\alpha\beta} + \mathcal{J}^{+0}_{-\boldsymbol{k},\beta\alpha}\right),
\end{aligned} \tag{S72}$$

where we have used the properties $\mathcal{J}^{0-}_{\boldsymbol{k},\alpha\beta} = \bar{\mathcal{J}}^{+0}_{\boldsymbol{k},\beta\alpha}$ and $\mathcal{J}^{0+}_{\boldsymbol{k},\alpha\beta} = \mathcal{J}^{+0}_{-\boldsymbol{k},\beta\alpha}$. We may then evaluate the derivatives of the spin-wave energies using Eqs. (S70,S72) as

$$\left(\frac{\partial\epsilon_{\boldsymbol{k},\alpha}}{\partial\lambda_\mu}\right)_0 = \boldsymbol{V}^{\dagger}_{\boldsymbol{k},\alpha}\begin{pmatrix}\boldsymbol{C}_{\boldsymbol{k},\mu} & \boldsymbol{D}_{\boldsymbol{k},\mu}\\ \boldsymbol{D}^{\dagger}_{\boldsymbol{k},\mu} & \boldsymbol{C}^{\intercal}_{-\boldsymbol{k},\mu}\end{pmatrix}\boldsymbol{V}_{\boldsymbol{k},\alpha}, \tag{S73}$$

where

$$\left[\boldsymbol{C}_{\boldsymbol{k},\mu}\right]_{\alpha\beta} \equiv \left(\frac{\partial\mathcal{J}^{+-}_{\boldsymbol{k},\alpha\beta}}{\partial\lambda_\mu}\right)_0, \quad \left[\boldsymbol{D}_{\boldsymbol{k},\mu}\right]_{\alpha\beta} \equiv \left(\frac{\partial\mathcal{J}^{++}_{\boldsymbol{k},\alpha\beta}}{\partial\lambda_\mu}\right)_0. \tag{S74}$$

The $K_{\mu\nu}$ term may then be evaluated as

$$K_{\mu\nu}(T) = \frac{S^2}{4TN}\sum_{\boldsymbol{k},\alpha}\boldsymbol{V}^{\dagger}_{\boldsymbol{k},\alpha}\begin{pmatrix}\boldsymbol{C}_{\boldsymbol{k},\mu} & \boldsymbol{D}_{\boldsymbol{k},\mu}\\ \boldsymbol{D}^{\dagger}_{\boldsymbol{k},\mu} & \boldsymbol{C}^{\intercal}_{-\boldsymbol{k},\mu}\end{pmatrix}\boldsymbol{V}_{\boldsymbol{k},\alpha}\boldsymbol{V}^{\dagger}_{\boldsymbol{k},\alpha}\begin{pmatrix}\boldsymbol{C}_{\boldsymbol{k},\nu} & \boldsymbol{D}_{\boldsymbol{k},\nu}\\ \boldsymbol{D}^{\dagger}_{\boldsymbol{k},\nu} & \boldsymbol{C}^{\intercal}_{-\boldsymbol{k},\nu}\end{pmatrix}\boldsymbol{V}_{\boldsymbol{k},\alpha}\,\mathrm{csch}^2\left(\frac{S\epsilon_{\boldsymbol{k},\alpha}}{2T}\right). \tag{S75}$$

This expression vanishes in the zero-temperature limit, that is $K_{\mu\nu} \to 0$ as $T \to 0^+$. The expression in Eq. (S75) is enormously useful as it involves only the linear spin-wave eigenvectors and exchange

matrices, and therefore circumvents the need to calculate derivatives of the spin-wave energies numerically (e.g. using a finite difference method).

We note the $\mathcal{J}^{+0}_{\boldsymbol{k},\alpha\beta}$ exchange couplings appearing in Eq. (S72) are directly related to the three-Magnon interaction vertices in Eq. (S7), given by

$$T^{\alpha\beta\mu}_{\boldsymbol{k}\boldsymbol{k}'} = -\delta_{\alpha\mu}\mathcal{J}^{+0}_{\boldsymbol{k}',\beta\alpha} - \delta_{\beta\mu}\mathcal{J}^{+0}_{\boldsymbol{k},\alpha\beta}. \tag{S76}$$

We may therefore conclude that if the spin-wave theory does not have any three-magnon, interactions, i.e. $\mathcal{T}^{\alpha\beta\mu}_{\boldsymbol{k}\boldsymbol{k}'} = 0$, then $K_{\mu\nu}(T) = 0$ and the PG gap can be calculated to $O(S^0)$ from the curvature of the linear spin-wave free energy. In the general case where three-body interactions are present, this additional term $K_{\mu\nu}(T)$ will be nonzero, however we emphasize that it still allows one to compute the PG gap within the framework of linear spin-wave theory.

## III. MODELS

We now discuss details of two additional magnetic pyrochlore materials, where the quantum spin models are known to exhibit ObD.

### A. $Yb_2Ge_2O_7$

First, we discuss the XY pyrochlore antiferromagnet $Yb_2Ge_2O_7$. Similar to the material $Er_2Ti_2O_7$ discussed in the main text, strong spin-orbit effects lead to a highly anisotropic (pseudo) spin-$\frac{1}{2}$ model

$$H = \sum_{\langle i,j\rangle}\Big[J_{zz}S^z_iS^z_j - J_{\pm}\left(S^+_iS^-_j + S^-_iS^+_j\right) + J_{\pm\pm}\left(\gamma_{ij}S^+_iS^+_j + \text{H.c.}\right) + J_{z\pm}\left(\zeta_{ij}\left[S^z_iS^+_j + S^+_iS^z_j\right] + \text{H.c.}\right)\Big], \tag{S77}$$

where $\gamma_{ij}, \zeta_{ij}$ are bond-dependent phase factors (see Ref. [8]). The four nearest-neighbor couplings have been fitted to inelastic neutron scattering data, with the best fit given by [9]

$$J_{zz} = 0.128\ \text{meV},\quad J_{\pm} = 0.138\ \text{meV},\quad J_{\pm\pm} = 0.044\ \text{meV},\quad J_{z\pm} = -0.188\ \text{meV}. \tag{S78}$$

The classical ground states are non-collinear antiferromagnetic configurations of spins lying in the local XY planes perpendicular to the local [111] cubic axes of the pyrochlore lattice [8], parametrized by an accidental $U(1)$ degeneracy [10]. Below $T_c \approx 0.572$ K [9], ObD selects one of the six "$\psi_3$" states, leading to a type I PG mode.

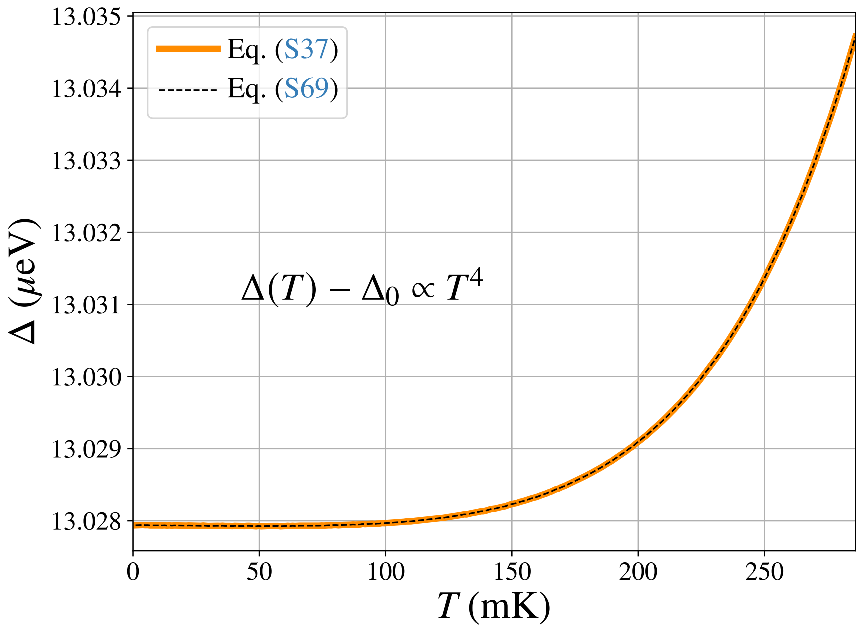


FIG. S1. PG gap for the pyrochlore antiferromagnet $Yb_2Ge_2O_7$, calculated using the exchange couplings from Ref. [9]. The classical ground states are parametrized by an accidental $U(1)$ degeneracy, corresponding to a type I mode. The gap is plotted up to $T_c/2 = 286$ mK.

The temperature dependence of PG gap for $Yb_2Ge_2O_7$ is depicted in Fig. S1 over a range of temperatures up to $T_c/2$. We find a zero-temperature contribution to the gap of $\Delta_0 = 13.028$ $\mu$eV, and a very small thermal correction of $\Delta(T_c/2) - \Delta_0 \approx 6$ neV. At low-temperature, the gap scales proportional to $T^4$ as expected for a type I mode.

### B. $Lu_2V_2O_7$

Finally, we discuss the somewhat unique scenario of the pyrochlore ferromagnet $Lu_2V_2O_7$. In this material, the $V^{4+}$ transition metal ions are magnetic, leading to the effective spin-$\frac{1}{2}$ model

$$H = -J \sum_{\langle i,j \rangle} \boldsymbol{S}_i \cdot \boldsymbol{S}_j - \sum_{\langle i,j \rangle} \boldsymbol{D}_{ij} \cdot (\boldsymbol{S}_i \times \boldsymbol{S}_j), \tag{S79}$$

where the DM vectors are of the "indirect" type [12]. The two nearest-neighbor couplings have been fitted to inelastic neutron scattering data, with the best fit given by [11]

$$J = 8.22 \text{ meV}, \qquad |\boldsymbol{D}_{ij}| = 1.5 \text{ meV}. \tag{S80}$$

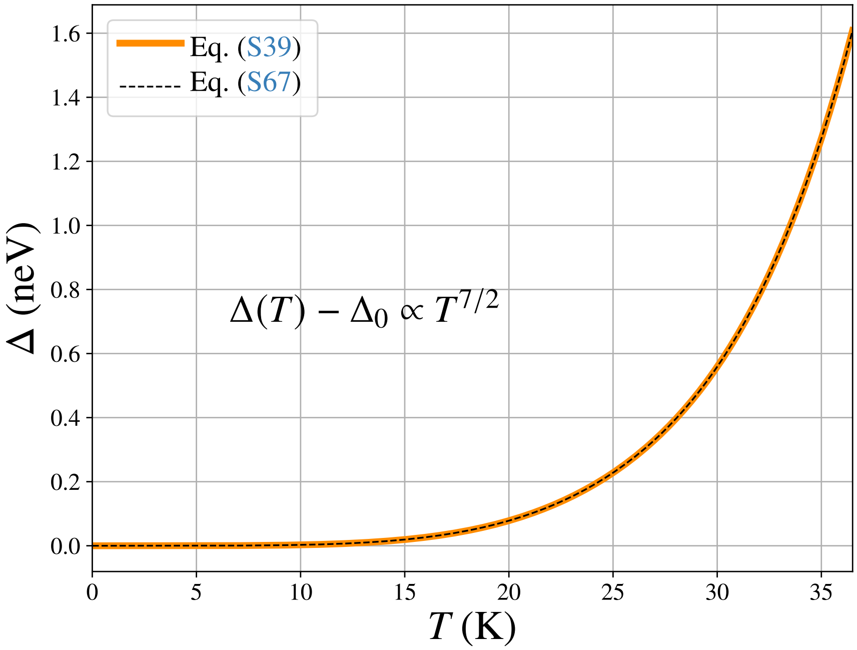


FIG. S2. PG gap for the pyrochlore ferromagnet $Lu_2V_2O_7$, calculated using the exchange couplings from Ref. [11]. The ground states are parametrized by an accidental $O(3)$ degeneracy, corresponding to a type II mode. The gap is plotted up to $T_c/2 = 36.5$ K.

The ground states are collinear ferromagnetic configurations parametrized by an accidental $O(3)$ degeneracy [13]. Below $T_c \approx 73$ K [11], ObD (within the model of Eq. (S79) selects one of the $\langle 111 \rangle$ directions for the bulk magnetization [13], leading to a type II PG mode.

The temperature dependence of the PG gap for $Lu_2V_2O_7$ is depicted in Fig. S2 over a range of temperatures up to $T_c/2$. In this case, there is no zero-temperature contribution to the gap, consistent with recent work in Ref. [13] arguing that this material exhibits ObD *without* quantum zero-point fluctuations. Moreover, we find at low-temperature a gap scales proportional to $T^{7/2}$, distinct from the expected $T^{5/2}$ scaling for a type II mode. This exception arises due to the observation pointed out in Ref. [13], that the anisotropy enters the spin-wave dispersion at $O(k^4)$ in the wavevector, when $|\boldsymbol{D}_{ij}| \ll J$. This implies the linear spin-wave free energy, at low-temperature, takes the form

$$f(\phi, \theta) = aT^{5/2} + b(\phi, \theta)T^{7/2} + O(T^{9/2}), \tag{S81}$$

with the coefficient $a$ being independent of the spin orientation. The $K_{\mu\nu}$ terms entering the curvature formula will have a similar low-temperature expansion, and Eq. (S67) is consistent with

this power-law scaling.

---


[1] J.-P. Blaizot and G. Ripka, *Quantum Theory of Finite Systems* (MIT Press, 1986).

[2] J. Colpa, Diagonalization of the quadratic boson hamiltonian, Phys. A: Stat. Mech. Appl. **93**, 327 (1978).

[3] H. Kondo, Y. Akagi, and H. Katsura, Non-Hermiticity and topological invariants of magnon Bogoliubov–de Gennes systems, Prog. Theor. Exp. Phys **2020**, 12A104 (2020).

[4] J. G. Rau, P. A. McClarty, and R. Moessner, Pseudo-Goldstone Gaps and Order-by-Quantum Disorder in Frustrated Magnets, Phys. Rev. Lett. **121**, 237201 (2018).

[5] E. Rastelli, *Statistical Mechanics of Magnetic Excitations: from Spin Waves to Stripes to Checkerboards* (World Scientific, London, 2013).

[6] G. D. Mahan, *Many-Particle Physics*, 3rd ed. (Springer New York, 2000).

[7] A. Altland and B. Simons, *Condensed Matter Field Theory*, 2nd ed. (Cambridge University Press, 2010).

[8] J. G. Rau and M. J. P. Gingras, Frustrated Quantum Rare-Earth Pyrochlores, Annual Review of Condensed Matter Physics **10**, 357 (2019).

[9] C. L. Sarkis, J. G. Rau, L. D. Sanjeewa, M. Powell, J. Kolis, J. Marbey, S. Hill, J. A. Rodriguez-Rivera, H. S. Nair, D. R. Yahne, S. Säubert, M. J. P. Gingras, and K. A. Ross, Unravelling competing microscopic interactions at a phase boundary: A single-crystal study of the metastable antiferromagnetic pyrochlore $Yb_2Ge_2O_7$, Phys. Rev. B **102**, 134418 (2020).

[10] H. Yan, O. Benton, L. Jaubert, and N. Shannon, Theory of multiple-phase competition in pyrochlore magnets with anisotropic exchange with application to $Yb_2Ti_2O_7$, $Er_2Ti_2O_7$, and $Er_2Sn_2O_7$, Phys. Rev. B **95**, 094422 (2017).

[11] M. Mena, R. S. Perry, T. G. Perring, M. D. Le, S. Guerrero, M. Storni, D. T. Adroja, C. Rüegg, and D. F. McMorrow, Spin-Wave Spectrum of the Quantum Ferromagnet on the Pyrochlore Lattice $Lu_2V_2O_7$, Phys. Rev. Lett. **113**, 047202 (2014).

[12] M. Elhajal, B. Canals, R. Sunyer, and C. Lacroix, Ordering in the pyrochlore antiferromagnet due to Dzyaloshinsky-Moriya interactions, Phys. Rev. B **71**, 094420 (2005).

[13] A. Hickey, D. Lozano-Gómez, and M. J. P. Gingras, Order-by-disorder without quantum zero-point fluctuations in the pyrochlore Heisenberg ferromagnet with Dzyaloshinskii-Moriya interactions, Phys.

Rev. B **111**, 184434 (2025).
